# Supplementary material for: Symbolic Verification of Cache Side-channel Freedom
Source: arXiv:1807.04701 source file (2018-07-12)
Supplement: Supplementary file 1 [file cachefix_supplement.pdf]

# Symbolic Verification of Cache Side-channel Freedom

## ABSTRACT

Cache timing attacks allow third-party observers to retrieve sensitive information from program executions. But, is it possible to automatically check the vulnerability of a program against cache timing attacks and then, automatically shield program executions against these attacks? For a given program, a cache configuration and an attack model, our CACHEFIX framework either verifies the cache side-channel freedom of the program or synthesizes a series of patches to ensure cache side-channel freedom during program execution. At the core of our framework is a novel symbolic verification technique based on automated abstraction refinement of cache semantics. The power of such a framework is to allow symbolic reasoning over counterexample traces and to combine it with runtime monitoring for eliminating cache side channels during program execution. Our evaluation with routines from OpenSSL, libfixedtimefixedpoint, GDK and FourQlib libraries reveals that our CACHEFIX approach (dis)proves cache side-channel freedom within an average of 75 seconds. Besides, in all except one case, CACHEFIX synthesizes *all* patches within 20 minutes to ensure cache side-channel freedom of the respective routines during execution.

## 1 INTRODUCTION

Cache timing attacks [23, 24] are among the most critical *side-channel attacks* [25] that retrieve sensitive information from program executions. Recent cache attacks [31] further show that cache side-channel attacks are practical even in commodity embedded processors, such as in ARM-based embedded platforms [31]. The basic idea of a cache timing attack is to observe the timing of cache hits and misses for a program execution. Subsequently, the attacker use such timing to guess the sensitive input via which the respective program was activated.

Given the practical relevance, it is crucial to verify whether a given program (*e.g.* an encryption routine) satisfies *cache side-channel freedom*, meaning the program *is not vulnerable* to cache timing attacks. However, verification of such a property is challenging for several reasons. Firstly, the verification of cache side-channel freedom requires a systematic integration of cache semantics within the program semantics. This, in turn, is based on the derivation of a suitable abstraction of cache semantics. Our proposed CACHEFIX approach automatically builds such an abstraction and systematically refines it until a proof of cache side-channel freedom is obtained or a real (*i.e.* non-spurious) counterexample is produced. Secondly, proving cache side-channel freedom of a program requires reasoning over multiple execution traces. To this end, we propose a symbolic verification technique within our CACHEFIX framework. Concretely, we capture the cache behaviour of a program via symbolic constraints over program inputs. Then, we leverage recent advances on *satisfiability modulo theory* (SMT) and constraint solving to (dis)prove the cache side-channel freedom of a program.

An appealing feature of our CACHEFIX approach is to employ symbolic reasoning over the real counterexample traces. To this end,

we systematically explore real counterexample traces and apply such symbolic reasoning to synthesize patches. Each synthesized patch captures a symbolic condition  $\nu$  on input variables and a sequence of actions that needs to be applied when the program is processed with inputs satisfying  $\nu$ . The application of a patch is guaranteed to reduce the channel capacity of the program under inspection. Moreover, if our checker terminates, then our CACHEFIX approach guarantees to synthesize all patches that *completely shields the program* against cache timing attacks [8, 14]. Intuitively, our CACHEFIX approach can start with a program  $\mathcal{P}$  vulnerable to cache timing attack. Then, it leverages a systematic combination of symbolic verification and runtime monitoring to execute  $\mathcal{P}$  with cache side-channel freedom.

It is the precision and the novel mechanism implemented within CACHEFIX that set us apart from the state of the art. Existing works on analyzing cache side channels [15, 22, 30] are incapable to automatically build and refine abstractions for cache semantics. Besides, these works are not directly applicable when the underlying program *does not* satisfy cache side-channel freedom. Given an arbitrary program, our CACHEFIX approach generates proofs of its cache side-channel freedom or generates input(s) that manifest the violation of cache side-channel freedom. Moreover, our symbolic reasoning framework provides capabilities to systematically synthesize patches and completely eliminate cache side channels during program execution.

We organize the remainder of the paper as follows. After providing an overview of CACHEFIX (Section 2), we make the following contributions:

- (1) We present CACHEFIX, a novel symbolic verification framework to check the cache side-channel freedom of an arbitrary program. To the best of our knowledge, this is the first application of automated abstraction refinement and symbolic verification to check the cache behaviour of a program.
- (2) We instantiate our CACHEFIX approach with direct-mapped caches, as well as with set-associative caches with *least recently used* (LRU) and *first-in-first-out* (FIFO) policy (Section 4.3). In Section 4.4, we show the generalization of our CACHEFIX approach over timing-based attacks [14] and trace-based attacks [8].
- (3) We discuss a systematic exploration of counterexamples to synthesize patches and to shield program executions against cache timing attacks (Section 5). We provide theoretical guarantees that such patch synthesis converges towards completely eliminating cache side channels during execution.
- (4) We provide an implementation of CACHEFIX and evaluate it with 25 routines from OpenSSL, GDK, FourQlib and libfixedtimefixedpoint libraries. Our evaluation reveals that CACHEFIX can establish proof or generate non-spurious counterexamples within 75 seconds on average. Besides, in most cases, CACHEFIX generated all patches within 20 minutes to ensure cache side-channel freedom during execution. Our implementation and all experimental data are publicly available.

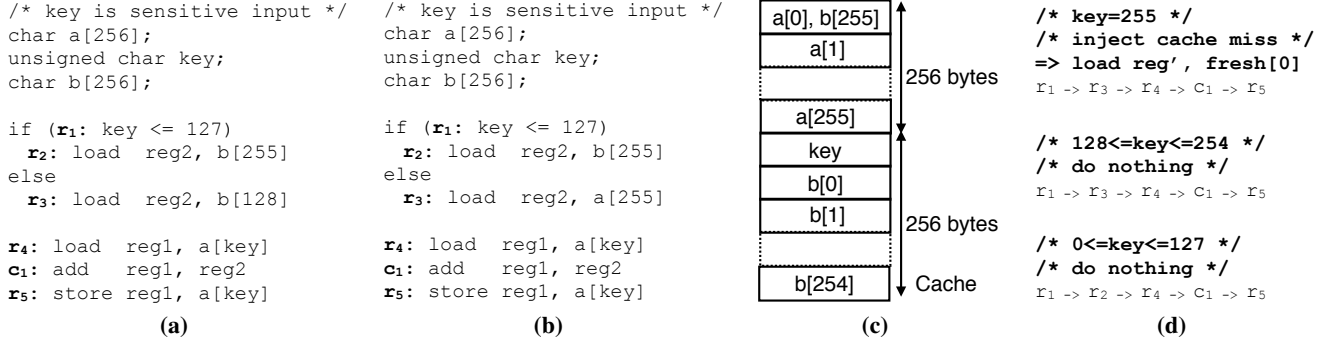

**Figure 1: A code fragment (a) satisfying cache side-channel freedom, (b) violating cache side-channel freedom. (c) Mapping of variables into the cache. (d) Runtime actions and the execution order for the program in Figure 1(b) to ensure cache side-channel freedom.**

## 2 OVERVIEW

In this section, we demonstrate the general insight behind our approach through examples. We consider the simple code fragments in Figure 1(a)-(b) where `key` is a sensitive input. For the sake of simplicity in this example, we will assume a direct-mapped cache having a size of 512 bytes. The mapping of different program variables into the cache appears in Figure 1(c). We assume the presence of an attacker who observes the number of cache misses in the victim program. Hence, the attacker can distinguish execution traces suffering different number of cache misses. With respect to such an attacker, the examples in Figure 1(a)-(b) satisfy cache side-channel freedom if and only if the number of cache misses suffered is independent of `key`. We propose an approach that verifies such property or generates a counterexample capturing its violation. As a byproduct of our verification, we also generate patches from the counterexamples to eliminate cache side channels.

**Positive example.** We first consider the example in Figure 1(a). Our CACHEFIX approach revolves around a systematic abstraction refinement of cache semantics. Starting with an initial abstraction of cache semantics (including the trivial empty abstraction), we systematically refine it to check the cache side-channel freedom of a program. Considering the example in Figure 1(a), its cache semantics can be accurately predicted via the following set of logical predicates:

$$\begin{aligned}
 Pred_{set} &= \{set(r_i) = set(r_j) \mid 1 \leq j < i \leq 5\} \\
 Pred_{tag} &= \{tag(r_i) \neq tag(r_j) \mid 1 \leq j < i \leq 5\}
 \end{aligned} \quad (1)$$

where  $set(r_i)$  and  $tag(r_i)$  captures the cache set and cache tag accessed by instruction  $r_i$ , respectively. In the following discussion, we abbreviate the predicate  $set(r_i) = set(r_j)$  via  $\rho_{ij}^{set}$  and the predicate  $tag(r_i) \neq tag(r_j)$  via  $\rho_{ij}^{tag}$ .

We symbolically execute the program in Figure 1(a). Subsequently, we convert both the program semantics and cache semantics into a symbolic formula  $\Psi$ . The conversion of cache semantics is based on the level of abstraction employed in  $Pred_{set} \cup Pred_{tag}$  (cf. Equation 1). We start with an abstraction of cache semantics where we only consider instructions with constant cache behaviours (i.e. independent of `key`). This includes instructions  $r_1$ ,  $r_2$  and  $r_3$ . To form such an initial abstraction, we identify predicates  $\rho_{12}^{set}, \rho_{13}^{set}, \rho_{23}^{set} \in Pred_{set}$  and predicates  $\rho_{12}^{tag}, \rho_{13}^{tag}, \rho_{23}^{tag} \in$

$Pred_{tag}$ . We call this initial set of predicates  $Pred_{init}$ . Any predicates  $p \in (Pred_{set} \cup Pred_{tag}) \setminus Pred_{init}$  are replaced with a fresh symbolic variable within the symbolic formula  $\Psi$ . Finally, we check the (un)satisfiability of  $\Psi$  against cache side-channel freedom.

Cache side-channel freedom of a program is a hyper-property, meaning that such a property requires reasoning of cache behaviour over multiple execution traces. Our symbolic reasoning integrates the cache semantics of a program within the symbolic formula  $\Psi$ . For each memory-related instruction  $r_i$ , the cache semantics are injected within  $\Psi$  as follows:

$$\Gamma(r_i) \Leftrightarrow (miss_i = 1); \neg \Gamma(r_i) \Leftrightarrow (miss_i = 0) \quad (2)$$

$miss_i$  is 1 if  $r_i$  is a cache miss and it is 0 otherwise.  $\Gamma(r_i)$  is a symbolic condition to capture the cache behaviour of  $r_i$  and it depends on our current level of abstraction. For instance, initially,  $\Gamma(r_i)$  explicitly includes predicates in  $Pred_{init}$ , but only contains placeholder symbolic variables for predicates in  $(Pred_{set} \cup Pred_{tag}) \setminus Pred_{init}$ .

Cache side-channel freedom holds for the program in Figure 1(a) when all feasible traces exhibit the same number of cache misses. Hence, such a property  $\varphi$  can be formulated as the non-existence of two traces  $tr_1$  and  $tr_2$  as follows:

$$\varphi \equiv \nexists tr_1, \nexists tr_2 \text{ s.t. } \left( \sum_{i=1}^5 miss_i^{(tr_1)} \neq \sum_{i=1}^5 miss_i^{(tr_2)} \right) \quad (3)$$

where  $miss_i^{(tr)}$  captures the valuation of  $miss_i$  in trace  $tr$ . In other words, we have the following verification goal:

$$\left| \Psi \wedge \left( \sum_{i=1}^5 miss_i \geq 0 \right) \right|_{sol(\sum_{i=1}^5 miss_i)} \leq 1 \quad (4)$$

The subscript  $sol(\sum_{i=1}^5 miss_i)$  captures the number of valuations of  $\sum_{i=1}^5 miss_i$ . Intuitively, we check whether  $\sum_{i=1}^5 miss_i$  has more than one valuation for Figure 1(a).

Our checker returns a violation of Equation 4 and provides counterexample traces  $tr_1$  and  $tr_2$  as follows.

$$tr_1 \equiv \langle miss_1 = miss_2 = miss_4 = 1, miss_3 = miss_5 = 0 \rangle$$

$$tr_2 \equiv \langle miss_1 = miss_3 = miss_4 = miss_5 = 1, miss_2 = 0 \rangle$$

Our further inspection reveals that  $tr_2$  is spurious. This is discovered by cross checking the valuation of  $miss_i$  variables with the cache semantics. Concretely, if  $miss_5 = 1$ , then  $\Gamma(r_5)$  must be satisfiable

(cf. Equation 2). However,  $\Gamma(r_5)$  is unsatisfiable with the following unsatisfiable core:

$$\mathcal{U} \equiv \neg \rho_{45}^{set} \vee \rho_{45}^{tag} \quad (5)$$

Recall that we replaced both  $\rho_{45}^{set}$  and  $\rho_{45}^{tag}$  with fresh symbolic variables in our initial abstraction. Intuitively, Equation 5 corresponds to the possibility that  $r_5$  can suffer a cold cache miss since  $r_4, r_5$  access different memory blocks. This is, however, impossible as  $r_4$  and  $r_5$  access the same memory block (i.e. both  $\rho_{45}^{set}$  and  $\neg \rho_{45}^{tag}$  are true). Given the unsatisfiable core  $\mathcal{U}$ , we refine our abstraction via including all predicates within  $\mathcal{U}$ . Hence, our refined abstraction include the following predicates from  $Pred_{tag} \cup Pred_{set}$ :  $\{\rho_{12}^{set}, \rho_{13}^{set}, \rho_{23}^{set}, \rho_{12}^{tag}, \rho_{13}^{tag}, \rho_{23}^{tag}, \rho_{45}^{set}, \rho_{45}^{tag}\}$ . With such a refined abstraction, we repeat the verification process and obtain the following counterexample traces:

$$tr'_1 \equiv \langle miss_1 = miss_2 = miss_4 = 1, miss_3 = miss_5 = 0 \rangle$$

$$tr'_2 \equiv \langle miss_1 = miss_3 = 1, miss_2 = miss_4 = miss_5 = 0 \rangle$$

Intuitively, our checker failed to see that  $r_4$  should be a cold cache miss in  $tr'_2$ , hence mistaking  $miss_4$  to be 0. This is due to the absence of predicates  $\{\rho_{14}^{set}, \rho_{14}^{tag}, \rho_{34}^{set}, \rho_{34}^{tag}\}$  in our current abstraction.

We continue the verification process in a similar fashion mentioned in the preceding. For our example in Figure 1(a), the process terminates when our checker proves the cache side-channel freedom with the following abstraction:

$$Pred_{cur} = \{\rho_{ij}^{set} \mid 1 \leq j < i \leq 4\} \cup \{\rho_{45}^{set}\} \\ \cup \{\rho_{ij}^{tag} \mid 1 \leq j < i \leq 4\} \cup \{\rho_{45}^{tag}\}$$

**Negative example.** We now consider the example shown in Figure 1(b) with the same initial abstraction:

$$\{\rho_{12}^{set}, \rho_{13}^{set}, \rho_{23}^{set}, \rho_{12}^{tag}, \rho_{13}^{tag}, \rho_{23}^{tag}\}$$

Our checker generates the following counterexample traces capturing the violation of cache side-channel freedom:

$$tr''_1 \equiv \langle miss_1 = miss_2 = miss_4 = 1, miss_3 = miss_5 = 0 \rangle$$

$$tr''_2 \equiv \langle miss_1 = miss_3 = 1, miss_2 = miss_4 = miss_5 = 0 \rangle$$

Further inspection reveals that both  $tr''_1$  and  $tr''_2$  are feasible. Hence, we have established that the program in Figure 1(b) does not satisfy cache side-channel freedom.

An appealing feature of our framework is to leverage verification results and automatically generate patches. Such patches aim to eliminate cache side channels of program. For instance, consider the feasible counterexamples  $tr''_1$  and  $tr''_2$ . Intuitively, our patching process changes all traces similar to  $tr''_2$  *on-the-fly* and makes them behave like  $tr''_1$ . Concretely,  $tr''_2$  will behave like  $tr''_1$ , with respect to the attacker, if we inject one cache miss to  $tr''_2$ . To this end, we need to compute all inputs that lead to counterexample trace  $tr''_2$ . Thanks to our symbolic reasoning framework (cf. Equation 2), we can compute a symbolic expression capturing all such inputs. For instance, since  $miss_4 = 0$ , we know  $\Gamma(r_4)$  must be false. Specifically, we have the following symbolic condition that captures all inputs leading to  $tr''_2$ :

$$v_1 \equiv \Gamma(r_1) \wedge \neg \Gamma(r_2) \wedge \Gamma(r_3) \wedge \neg \Gamma(r_4) \wedge \neg \Gamma(r_5)$$

$v_1$  is satisfiable if and only if  $key = 255$ . Hence, we inject a cache miss whenever the code in Figure 1(b) is executed with inputs satisfying  $v_1$ , i.e., for input  $key = 255$  (cf. Figure 1(d)).

We continue the verification process to reveal all other counterexamples violating cache side-channel freedom. To this end, we aim to only find unique counterexamples. Hence, we modify the symbolic formula  $\Psi$  to  $\Psi \wedge \neg v_1$  and aim to satisfy the following verification goal:

$$\left| \Psi \wedge \neg v_1 \wedge \left( \left( \sum_{i=1}^5 miss_i \right) \geq 0 \right) \right|_{sol(\sum_{i=1}^5 miss_i)} \leq 1 \quad (6)$$

Our checker goes through a series of abstraction refinement and reveals that Equation 6 holds for the program in Figure 1(b). At this stage, our checker terminates with exactly one patch to be applied for inputs satisfying  $v_1 \equiv (key = 255)$ .

### 3 SIDE-CHANNEL CHECKER WORKFLOW

**Threat Model.** We assume that an attacker makes observations on the execution traces of victim program  $\mathcal{P}$  and the implementation of  $\mathcal{P}$  is known to the attacker. Besides, there does not exist any *error* in the observations made by the attacker. We also assume that an attacker can execute arbitrary user-level code on the processor that runs the victim program. This, in turn, allows the attacker to flush the cache (e.g. via accessing a large array) before the victim routine starts execution. We, however, do not assume that the attacker can access the address space of the victim program  $\mathcal{P}$ . We believe the aforementioned assumptions on the attacker are justified, as we aim to verify the cache side-channel freedom of programs against *strong attacker models*.

We capture an execution trace via a sequence of hits ( $h$ ) and misses ( $m$ ). Hence, formally we model an attacker as the mapping  $O : \{h, m\}^* \rightarrow \mathbb{X}$ , where  $\mathbb{X}$  is a countable set. For  $tr_1, tr_2 \in \{h, m\}^*$ , an attacker can distinguish  $tr_1$  from  $tr_2$  if and only if  $O(tr_1) \neq O(tr_2)$ . In this paper, we instantiate our checker for the following realistic attack models:

- $O_{time} : \{h, m\}^* \rightarrow \mathbb{N}$ .  $O_{time}$  maps each execution trace to the number of cache misses suffered by the same. This attack model imitates cache timing attacks [14].
- $O_{trace} : \{h, m\}^* \rightarrow \{0, 1\}^*$ .  $O_{trace}$  maps each execution trace to a bitvector ( $h$  is mapped to 0 and  $m$  is mapped to 1). This attack model imitates trace-based attacks [8].

**Overview of CacheFix.** The key novelty in our framework (cf. Figure 2) is two fold: Firstly, we provide capabilities to automatically refine the abstraction for cache semantics (see Section 4 for details). This is accomplished with the goal of proving cache side-channel freedom of an arbitrary program. Secondly, we leverage the real counterexamples generated during the verification process to automatically synthesize patches. These patches can be applied at runtime and they are guaranteed to increase the uncertainty to guess sensitive inputs (see Section 5 for details). Given a program  $\mathcal{P}$  and an attacker model  $O$ , our checker first builds an initial abstraction  $Pred_{init}$ . With this abstraction, our checker either verifies the cache side-channel freedom or produces a counterexample. If a spurious counterexample is found, we *automatically* refine  $Pred_{init}$  and repeat the verification process. This refinement process is guaranteed

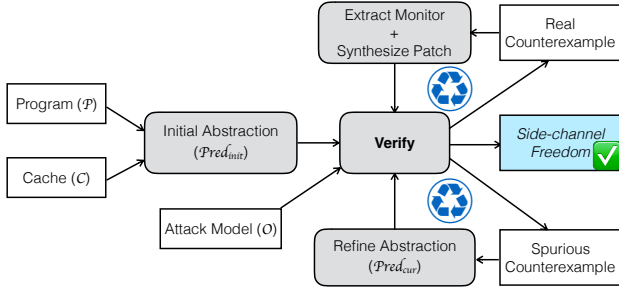

Figure 2: Workflow of our symbolic verification and patching

to converge towards the most precise abstraction of cache semantics to (dis)prove the cache side-channel freedom of  $\mathcal{P}$ .

An appealing feature of our checker is the usage of real counterexamples to synthesize patches. Concretely, if a real counterexample is found, then  $\mathcal{P}$  does not satisfy cache side-channel freedom. Hence, we generate patches that can be applied at runtime and these patches drive  $\mathcal{P}$  to satisfy the cache side-channel freedom property during execution. To this end, we extract a monitor from a real counterexample. Such a monitor captures a symbolic condition on input variables for which the same patch can be applied. For timing-based attacks [14], each monitor captures a symbolic condition  $v$  on input variables and each patch captures a time-delay  $\tau$  that needs to be injected for inputs  $I$  satisfying  $v$ . We repeat the process of verification and patch generation until all real counterexamples are patched. We note that such a process may never terminate. However, the patch-synthesis process guarantees to increase the uncertainty of guessing sensitive inputs of  $\mathcal{P}$ . Moreover, upon termination, our checker guarantees  $\mathcal{P}$  to satisfy cache side-channel freedom, should all synthesized patches are applied during the execution of  $\mathcal{P}$ .

## 4 ABSTRACTION REFINEMENT FOR VERIFICATION

**Processor model.** We assume an ARM-style processor with one or more cache levels. However, we consider timing attacks only due to first-level instruction or data caches [8, 14]. We currently do not handle more advanced attacks on shared caches [32]. First-level caches can either be partitioned (instruction vs. data) or unified. We assume that set-associative caches have either LRU or FIFO replacement policy. Other deterministic replacement policies can easily be integrated within CACHEFIX via additional symbolic constraints. Finally, our timing model only takes into account the effect of caches. Timing effects due to other micro-architectural features (e.g. pipeline and branch prediction) are currently not handled. For the sake of brevity, we discuss the timing effects due to memory-related instructions. It is straightforward to integrate the timing effects of computation instructions (e.g. add) into CACHEFIX.

**Notations.** We represent cache via a triple  $\langle 2^S, 2^B, \mathcal{A} \rangle$  where  $2^S$ ,  $2^B$  and  $\mathcal{A}$  capture the number of cache sets, cache line size and cache associativity, respectively. We use  $set(r_i)$  and  $tag(r_i)$  to capture the cache set and cache tag, respectively, accessed by instruction  $r_i$ . Additionally, we introduce a symbolic variable  $miss_i$  to capture the hit/miss classification of instruction  $r_i$ .  $miss_i$  is set to 1 if  $r_i$  is a cache miss, otherwise it is set to 0. For instructions  $r_i$

and  $r_j$ , we have  $j < i$  if and only if  $r_j$  was (symbolically) executed before  $r_i$ .

### 4.1 Initial abstract domain

We assume that a routine may start execution with any initial cache state, but it does not access memory blocks within the initial state during execution [22]. Hence, for a given instruction  $r_i$ , its cache behaviour might be affected by all instructions executing prior to  $r_i$ . Concretely, the cache behaviour of  $r_i$  can be accurately predicted based on the set of logical predicates  $Pred_{set}$  and  $Pred_{tag}$  as follows:

$$\begin{aligned} Pred_{set}^i &= \{set(r_j) = set(r_i) \mid 1 \leq j < i\} \\ Pred_{tag}^i &= \{tag(r_j) \neq tag(r_i) \mid 1 \leq j < i\} \end{aligned} \quad (7)$$

Intuitively,  $Pred_{set}^i$  captures the set of predicates checking whether any instruction prior to  $r_i$  accesses the same cache set as  $r_i$ . Similarly,  $Pred_{tag}^i$  checks whether any instruction prior to  $r_i$  has a different cache tag than  $tag(r_i)$ . Based on this intuition, the following set of predicates are sufficient to predict the cache behaviours of  $N$  memory-related instructions.

$$Pred_{set} = \bigcup_{i=1}^N Pred_{set}^i; \quad Pred_{tag} = \bigcup_{i=1}^N Pred_{tag}^i \quad (8)$$

Analyzing all predicates in  $Pred_{tag} \cup Pred_{set}$  may be cumbersome for programs with complex data/control flow. Hence, we launch verification with a smaller set of predicates  $Pred_{init} \subseteq Pred_{tag} \cup Pred_{set}$ .  $Pred_{init}$  is computed as follows:

$$\begin{aligned} Pred_{init} &= \bigcup_{i=1}^N \{p \mid p \in Pred_{tag} \cup Pred_{set} \wedge |\sigma(r_i)| = 1 \wedge \\ &\quad \forall k \in [1, i). |\sigma(r_k)| = 1 \wedge guard_k \Rightarrow true\} \end{aligned} \quad (9)$$

$\sigma(r_i)$  captures the set of memory blocks accessed by instruction  $r_i$  and  $guard_k$  captures the control condition under which  $r_k$  is executed. Intuitively,  $Pred_{init}$  contains a set of predicates that are guaranteed to be input independent. We note that  $guard_k$  depends on the program semantics. The abstraction of program semantics is an orthogonal problem and for the sake of brevity, we skip its discussion here. In the next section, we discuss the mechanism to use and refine  $Pred_{init}$  for proving the cache side-channel freedom of an arbitrary program.

### 4.2 Abstract domain refinement

We use the mapping  $\Gamma : \{r_1, r_2, \dots, r_N\} \rightarrow \{true, false\}$  to capture the conditions under which  $r_i$  was a cache hit or a cache miss. In particular, the following relationships hold:

$$\Gamma(r_i) \Leftrightarrow (miss_i = 1); \quad \neg \Gamma(r_i) \Leftrightarrow (miss_i = 0) \quad (10)$$

$miss_i$  is 1 if  $r_i$  suffers a cache miss and  $miss_i$  is 0 otherwise. Clearly  $\Gamma(r_i)$  depends on predicates in  $Pred_{set}^i \cup Pred_{tag}^i$ .

**ExecuteSymbolic.** Algorithm 1 captures the overall verification process based on our systematic abstraction refinement. The symbolic verification engine computes a formula representation  $\Psi$  of the program  $\mathcal{P}$ . This is accomplished via a symbolic execution on program  $\mathcal{P}$  (cf. procedure EXECUTESYMBOLIC) and systematically translating the cache and program semantics of each instruction into a set of constraints (cf. procedure CONVERT).

**Algorithm 1** Abstraction Refinement Algorithm

---

**Input:** Program  $\mathcal{P}$ , cache configuration  $C$ , attack model  $\mathcal{O}$   
**Output:** Successful verification or a concrete counterexample

```

1: /*  $\Psi$  is a formula representation of  $\mathcal{P}$  */
2: /*  $Pred$  is cache-semantics-related predicates */
3: /*  $\Gamma$  determines cache behaviour of all instructions */
4:  $(\Psi, Pred, \Gamma) := \text{EXECUTESYMBOLIC}(\mathcal{P}, C)$ 
5: /* Formulate initial abstraction (cf. Equation 9) */
6:  $Pred_{cur} := Pred_{init} := \text{GETINITIALABSTRACTION}(Pred)$ 
7: /* Rewrite  $\Psi$  with initial abstraction */
8:  $\text{REWRITE}(\Psi, Pred_{init})$ 
9: /* Formulate cache side-channel freedom property */
10:  $\varphi := \text{GETPROPERTY}(\mathcal{O})$ 
11: /* Invoke symbolic verification to check  $\Psi \wedge \neg\varphi$  */
12:  $(res, tr_1, tr_2) := \text{VERIFY}(\Psi, \varphi)$ 
13: while  $(res = false) \wedge (tr_1 \text{ or } tr_2 \text{ is spurious})$  do
14:   /* Extract unsatisfiable core from  $tr_1$  and/or  $tr_2$  */
15:    $\mathcal{U} := \text{UNSATCORE}(tr_1, tr_2, \Gamma)$ 
16:   /* Refine abstractions and repeat verification */
17:    $Pred_{cur} := \text{REFINE}(Pred_{init}, \mathcal{U}, Pred)$ 
18:    $\text{REWRITE}(\Psi, Pred_{cur})$ 
19:    $(res, tr_1, tr_2) := \text{VERIFY}(\Psi, \varphi)$ 
20:    $Pred_{init} := Pred_{cur}$ 
21: end while
22: return  $res$ 

```

---

**Procedure 2** Symbolically Tracking Program and Cache States

---

```

1: /* symbolically execute  $\mathcal{P}$  with cache configuration  $C$  */
2: procedure  $\text{EXECUTESYMBOLIC}(\mathcal{P}, C)$ 
3:    $i := 1; \Psi := true; Pred_{set} := Pred_{tag} := \phi$ 
4:    $r_i := \text{GETNEXTINSTRUCTION}(\mathcal{P})$ 
5:   while  $r_i \neq \text{exit}$  do
6:     if  $r_i$  is memory-related instruction then
7:       /* Collect predicates for cache semantics */
8:        $Pred_{set} \cup = Pred_{set}^i; Pred_{tag} \cup = Pred_{tag}^i$ 
9:       /*  $\Gamma(r_i)$  determines cache behaviour of  $r_i$  */
10:      Formulate  $\Gamma(r_i)$  /* see Section 4.3 */
11:       $\Gamma \cup = \{\Gamma(r_i)\}$ 
12:      /* Integrate cache semantics within  $\Psi$  */
13:       $\Psi := \text{CONVERT}(\Psi, \Gamma(r_i) \Leftrightarrow (miss_i = 1))$ 
14:       $\Psi := \text{CONVERT}(\Psi, \neg\Gamma(r_i) \Leftrightarrow (miss_i = 0))$ 
15:    end if
16:    /* Integrate program semantics of  $r_i$  within  $\Psi$  */
17:    /*  $\varphi(r_i)$  is a predicate capturing  $r_i$  semantics */
18:     $\Psi := \text{CONVERT}(\Psi, \varphi(r_i))$ 
19:     $i := i + 1$ 
20:     $r_i := \text{GETNEXTINSTRUCTION}(\mathcal{P})$ 
21:  end while
22:  return  $(\Psi, Pred_{set} \cup Pred_{tag}, \Gamma)$ 
23: end procedure

```

---

**Convert.** During the symbolic execution, a set of symbolic states, each capturing a unique execution path reaching an instruction  $r_i$ , is maintained. This set of symbolic states can be viewed as a disjunction  $\Psi(r_i) \equiv \psi_1 \vee \psi_2 \vee \dots \vee \psi_{j-1} \vee \psi_j$ , where  $\Psi(r_i) \Rightarrow \Psi$  and

each  $\psi_i$  symbolically captures a unique execution path leading to instruction  $r_i$ . At each instruction  $r_i$ , the procedure **CONVERT** translates  $\Psi(r_i)$  in such a fashion that  $\Psi(r_i)$  integrates both the cache semantics (cf. lines 13-14) and program semantics (cf. lines 18) of  $r_i$ . For instance, to integrate cache semantics of a memory-related instruction  $r_i$ ,  $\Psi(r_i)$  is converted to  $\Psi(r_i) \wedge (\Gamma(r_i) \Leftrightarrow (miss_i = 1)) \wedge (\neg\Gamma(r_i) \Leftrightarrow (miss_i = 0))$ . Similarly, the program semantics of instruction  $r_i$ , as captured via  $\varphi(r_i)$ , is integrated within  $\Psi(r_i)$  as  $\Psi(r_i) \wedge \varphi(r_i)$ . Translating the *program semantics* of each instruction to a set of constraints is a standard technique in any symbolic model checking [19]. Moreover, such a translation is typically carried out on a program in static single assignment (SSA) form and takes into account both data and control flow. Unlike classic symbolic analysis, however, we consider both the cache semantics and program semantics of an execution path, as explained in the preceding.

**GetInitialAbstraction.** We start our verification with an initial abstraction of cache semantics (cf. Equation 9). Such an initial abstraction contains a partial set of logical predicates  $Pred_{init} \subseteq Pred_{set} \cup Pred_{tag}$ . Based on  $Pred_{init}$ , we rewrite  $\Psi$  via the procedure **REWRITE** as follows: We walk through  $\Psi$  and look for occurrences of any predicate  $p^- \in (Pred_{set} \cup Pred_{tag}) \setminus Pred_{init}$ . For any  $p^-$  discovered in  $\Psi$ , we replace  $p^-$  with a fresh symbolic variable  $V_{p^-}$ . Intuitively, this means that during the verification process, we assume any truth value for the predicates in  $(Pred_{set} \cup Pred_{tag}) \setminus Pred_{init}$ . This, in turn, substantially reduces the size of the symbolic formula  $\Psi$  and simplifies the verification process.

**Verify and GetProperty.** The procedure **VERIFY** invokes the solver to check the cache side-channel freedom of  $\mathcal{P}$  with respect to attack model  $\mathcal{O}$ . The property  $\varphi$ , capturing the cache side-channel freedom, is computed via **GETPROPERTY**. For timing-based attacks, such a property can be specified as follows:

$$\varphi \equiv \nexists tr_1, \nexists tr_2 \text{ s.t. } \left( \sum_{i=1}^{N[tr_1]} miss_i^{(tr_1)} \neq \sum_{i=1}^{N[tr_2]} miss_i^{(tr_2)} \right) \quad (11)$$

$miss_i^{(tr)}$  is the valuation of  $miss_i$  in trace  $tr$ .  $N[tr_1]$  and  $N[tr_2]$  capture the number of memory-related instructions in traces  $tr_1$  and  $tr_2$ , respectively. In Equation 11, the side-channel freedom is captured by the non-existence of any two traces  $tr_1$  and  $tr_2$  that have different number of cache misses. In practice, if the following formula is satisfied with more than one valuations for  $\sum_{i=1}^N miss_i$ , then side-channel freedom is violated:

$$\Psi \wedge \left( \left( \sum_{i=1}^N miss_i \right) \geq 0 \right) \quad (12)$$

Here  $N$  captures the total number of memory-related instructions encountered during the symbolic execution of  $\mathcal{P}$ .

**Refine and Rewrite.** If our verification process fails, we extract counterexample traces  $tr_1, tr_2$  with the current level of abstraction. Such counterexamples capture the valuation of all symbolic variables in the formula  $\Psi$ . To check the feasibility of  $trace \in \{tr_1, tr_2\}$ , we need to check whether valuations of all the symbolic variables in  $trace$  are feasible. To this end, we extract the valuation of  $miss_i$  for each memory-related instruction  $r_i$ . Recall from Equation 10 that  $\Gamma(r_i)$  accurately captures the set of conditions to determine the cache

behaviour of  $r_i$ . Therefore,  $r_i$  is a cache miss if and only if  $\Gamma(r_i)$  is *true*. We leverage this relation to construct the following formula  $\Gamma_{trace}$  for feasibility checking:

$$\Gamma_{trace} = \bigwedge_{i=1}^N \begin{cases} \Gamma(r_i), & \text{if } \text{miss}_i^{(trace)} = 1; \\ \neg\Gamma(r_i), & \text{if } \text{miss}_i^{(trace)} = 0; \end{cases} \quad (13)$$

In Equation 13,  $\text{miss}_i^{(trace)}$  captures the valuation of symbolic variable  $\text{miss}_i$  in the counterexample  $trace$ . We note that  $trace$  is not a spurious counterexample if and only if  $\Gamma_{trace}$  is *satisfiable*, hence, highlighting the violation of cache side-channel freedom.

If  $\Gamma_{trace}$  is *unsatisfiable*, then we have discovered a spurious counterexample. Intuitively, it means that our initial abstraction  $Pred_{init}$  was insufficient to (dis)prove the cache side-channel freedom. In order to refine this abstraction, we extract the *unsatisfiable core* from the symbolic formula  $\Gamma_{trace}$  via the procedure UNSAT-CORE. Such an unsatisfiable core contains a set of CNF clauses  $\in \bigcup_{k \in [1, N]} \Gamma(r_k)$ . We note each  $\Gamma(r_k)$  is a function of the set of predicates  $Pred_{tag} \cup Pred_{set}$ . Hence, in the unsatisfiable core of  $\Gamma_{trace}$ , we identify all predicates  $p^+ \in (Pred_{tag} \cup Pred_{set}) \setminus Pred_{init}$ . Subsequently, we refine the abstraction (cf. procedure REFINE in Algorithm 1) by including all such predicates. Concretely, we have a refined abstraction  $Pred_{cur}$  as follows:

$$Pred_{cur} := Pred_{init} \cup \{p^+ \mid p^+ \in \text{UnsatCore}(\Gamma_{trace}) \wedge p^+ \notin Pred_{init}\} \quad (14)$$

With the refined abstraction  $Pred_{cur}$ , we rewrite the symbolic formula  $\Psi$  (cf. procedure REWRITE). In particular, we identify the placeholder symbolic variables for predicates in the set  $Pred_{cur} \setminus Pred_{init}$ . We rewrite  $\Psi$  by replacing these placeholder symbolic variables with the respective predicates in the set  $Pred_{cur} \setminus Pred_{init}$ . It is worthwhile to note that the placeholder symbolic variables in  $(Pred_{tag} \cup Pred_{set}) \setminus Pred_{cur}$  remain unchanged.

**Termination.** The verification process is repeated with each iteration of abstraction refinement. As seen in Algorithm 1, the verification process continues until a real counterexample is produced or the side-channel freedom property is proved.

### 4.3 Modeling Cache Semantics

For each memory-related instruction  $r_i$ , the formulation of  $\Gamma(r_i)$  is critical to prove the cache side-channel freedom. The formulation of  $\Gamma(r_i)$  depends on the configuration of caches. Due to space constraints, we will only discuss the symbolic model for direct-mapped caches (symbolic models for LRU and FIFO caches are provided in the supplement [7]). Nevertheless, CACHEFIX also encodes the semantics of set-associative caches with least-recently-used (LRU) and first-in-first-out (FIFO) replacement policies. Hence, CACHEFIX can be used to evaluate the cache side-channel freedom for a variety of cache configurations.

To simplify the formulation, we will use the following abbreviations for the rest of the section:

$$\rho_{ij}^{set} \equiv (set(r_i) = set(r_j)); \quad \rho_{ij}^{tag} \equiv (tag(r_i) \neq tag(r_j)) \quad (15)$$

We also distinguish between the following variants of misses:

- (1) **Cold misses:** Cold misses occur when a memory block is accessed for the first time.

- (2) **Conflict misses:** All cache misses that are not cold misses are referred to as conflict misses.

**Formulating conditions for cold misses.** Cold cache misses occur when a memory block is accessed for the *first time during program execution*. In order to check whether  $r_i$  suffers a cold miss, we check whether all instructions  $r \in \{r_1, r_2, \dots, r_{i-1}\}$  access different memory blocks than the memory block accessed by  $r_i$ . This is captured as follows:

$$\Theta_i^{cold} \equiv \bigwedge_{j \in [1, i)} (\neg \rho_{ji}^{set} \vee \rho_{ji}^{tag} \vee \neg guard_j) \quad (16)$$

Recall that  $guard_j$  captures the control condition under which  $r_j$  is executed. Hence, if  $guard_j$  is evaluated false for a trace, then  $r_j$  does not appear in the respective trace. If  $\Theta_i^{cold}$  is satisfied, then  $r_i$  inevitably suffers a cold cache miss.

**Formulating conditions for conflict cache misses.** For direct-mapped caches, an instruction  $r_i$  suffers a conflict miss due to an instruction  $r_j$  if all of the following conditions are satisfied:

$\phi_{ji}^{cnf, dir}$ : If  $r_j$  accesses the same cache set as  $r_i$ , however,  $r_j$  accesses a different cache tag as compared to  $r_i$ . This is formally captured as follows:

$$\phi_{ji}^{cnf, dir} \equiv \rho_{ji}^{tag} \wedge \rho_{ji}^{set} \quad (17)$$

$\phi_{ji}^{rel, dir}$ : No instruction between  $r_j$  and  $r_i$  accesses the same memory block as  $r_i$ . For instance, consider the memory-block access sequence  $(r_1 : m_1) \rightarrow (r_2 : m_2) \rightarrow (r_3 : m_2)$ , where both  $m_1$  and  $m_2$  are mapped to the same cache set and  $r_{1..3}$  captures the respective memory-related instructions. It is not possible for  $r_1$  to inflict a conflict miss for  $r_3$ , as the memory block  $m_2$  is reloaded by instruction  $r_2$ .  $\phi_{ji}^{rel, dir}$  is formally captured as follows:

$$\phi_{ji}^{rel, dir} \equiv \bigwedge_{j < k < i} (\rho_{ki}^{tag} \vee \neg \rho_{ki}^{set} \vee \neg guard_k) \quad (18)$$

Intuitively,  $\phi_{ji}^{rel, dir}$  captures that all instructions between  $r_j$  and  $r_i$  either access a different memory block than  $r_i$  (hence, satisfying  $\rho_{ki}^{tag} \vee \neg \rho_{ki}^{set}$ ) or does not appear in the execution trace (hence, satisfying  $\neg guard_k$ ).

Given the intuition mentioned in the preceding paragraphs, we conclude that  $r_i$  suffers a conflict miss if both  $\phi_{ji}^{cnf, dir}$  and  $\phi_{ji}^{rel, dir}$  are satisfied for *any instruction executing prior to*  $r_i$ . This is captured in the symbolic condition  $\Theta_i^{cnf, dir}$  as follows:

$$\Theta_i^{cnf, dir} \equiv \bigvee_{j \in [1, i)} (\phi_{ji}^{cnf, dir} \wedge \phi_{ji}^{rel, dir} \wedge guard_j) \quad (19)$$

**Computing  $\Gamma(r_i)$ .** For direct-mapped caches,  $r_i$  can be a cache miss if it is either a cold cache miss or a conflict miss. Hence,  $\Gamma(r_i)$  is captured symbolically as follows:

$$\Gamma(r_i) \equiv guard_i \wedge (\Theta_i^{cold} \vee \Theta_i^{cnf, dir}) \quad (20)$$

### 4.4 Property for cache side-channel freedom

In this paper, we instantiate our checker for timing-based attacks [14] and trace-based attacks [8] as follows.

**Timing-based attacks.** In timing-based attacks, an attacker aims to distinguish traces based on their timing. Therefore, as shown in Equation 11, such a property can be formalized via the existence of two traces where the summation of cache misses differ. In our framework, we verify the following property to ensure cache side-channel freedom:

$$\left| \Psi \wedge \left( \sum_{i=1}^N \text{miss}_i \geq 0 \right) \right|_{\text{sol}(\sum_{i=1}^N \text{miss}_i)} \leq 1 \quad (21)$$

$N$  captures the number of symbolically executed, memory-related instructions.  $\text{sol}(\sum_{i=1}^N \text{miss}_i)$  captures the number of valuations of  $\sum_{i=1}^N \text{miss}_i$ . Intuitively, Equation 21 aims to check that the underlying program has exactly one cache behaviour, in terms of the total number of cache misses.

**Trace-based attacks.** In trace-based attacks, an attacker monitors the cache behaviour of each memory access. We define a partial function  $\xi : \{r_1, \dots, r_N\} \rightarrow \{0, 1\}$  as follows:

$$\xi(r_i) = \begin{cases} 1, & \text{if } \text{guard}_i \wedge (\text{miss}_i = 1) \text{ holds;} \\ 0, & \text{if } \text{guard}_i \wedge (\text{miss}_i = 0) \text{ holds;} \end{cases} \quad (22)$$

The following verification goal ensures side-channel freedom:

$$\left| \Psi \wedge |\text{dom}(\xi)| \geq 0 \wedge (\|_{r_i \in \text{dom}(\xi)} \xi(r_i)) \geq 0 \right|_{\text{sol}(X)} \leq 1 \quad (23)$$

where  $\text{dom}(\xi)$  captures the domain of  $\xi$ ,  $\|$  captures the ordered (with respect to the indexes of  $r_i$ ) concatenation operation and  $X = \langle |\text{dom}(\xi)|, \|_{r_i \in \text{dom}(\xi)} \xi(r_i) \rangle$ . Intuitively, we check whether there exists exactly one cache behaviour sequence.

## 5 RUNTIME MONITORING

CACHEFIX produces the first real counterexample when it discovers two traces with different observations (w.r.t. attack model  $\mathcal{O}$ ). These traces are then analyzed to compute a set of runtime actions that are guaranteed to reduce the channel capacity of the program. Overall, our runtime monitoring involves the following crucial steps:

- We analyze a counterexample trace  $tr$  and extract the symbolic condition for which the same counterexample trace  $tr$  would be generated,
- We systematically explore unique counterexamples with the objective to monotonically reduce the channel capacity of the program,
- We compute a set of runtime actions that need to be applied for improving the cache side-channel freedom.

In the following, we discuss these three steps in more detail.

**Analyzing a counterexample trace.** Given a real counterexample trace, we extract a symbolic condition that captures all the inputs for which the same counterexample trace can be obtained. Thanks to the symbolic nature of our analysis, CACHEFIX already includes capabilities to extract these monitors as follows.

$$v \equiv \bigwedge_{i=1}^{N_{\text{trace}}} \begin{cases} \Gamma(r_i), & \text{if } \text{miss}_i^{(\text{trace})} = 1; \\ \neg \Gamma(r_i), & \text{if } \text{miss}_i^{(\text{trace})} = 0; \end{cases} \quad (24)$$

where  $N_{\text{trace}}$  is the number of memory-related instructions in  $\text{trace}$  and  $\text{miss}_i^{(\text{trace})}$  is the valuation of symbolic variable  $\text{miss}_i$  in  $\text{trace}$ .

Once we extract a monitor  $v$  from counterexample trace, the symbolic system  $\Psi$  is refined to  $\Psi \wedge \neg v$ . This is to ensure that we only explore unique counterexample traces.

**Systematic exploration of counterexamples.** The order of exploring counterexamples is crucial to satisfy *monotonicity*, i.e., to reduce the channel capacity of program  $\mathcal{P}$  with each round of patch generation. To this end, CACHEFIX employs a strategy that can be visualized as an exploration of the equivalence classes of observations (e.g. #cache misses), i.e., we explore all counterexamples in the same equivalence class in one shot. In order to find another counterexample exhibiting the same observation as observation  $o$ , we modify the verification goal as follows, for timing and trace-based attacks, respectively (cf. Equation 22 for  $\xi$ ):

$$\begin{aligned} & \Psi \wedge \neg \left( \left( \sum_{i=1}^N \text{miss}_i \right) \neq o \right); \\ & \Psi \wedge \neg \left( \vee \left( \begin{aligned} & |\text{dom}(\xi)| \neq [|\text{dom}(\xi)|]_o \\ & \vee \|_{r_i \in \text{dom}(\xi)} \xi(r_i) \neq [\|_{r_i \in \text{dom}(\xi)} \xi(r_i)]_o \end{aligned} \right) \right) \end{aligned} \quad (25)$$

where  $[X]_o$  captures the valuation of  $X$  with respect to observation  $o$  and  $N$  is the total number of symbolically executed, memory-related instructions. If Equation 25 is unsatisfiable, then it captures the absence of any more counterexample with the observation  $o$ . It is worthwhile to note that  $\Psi$  is automatically refined so that we do not discover the same counterexample twice. If Equation 25 is satisfiable, our checker provides another non-spurious counterexample with the observation  $o$ . We repeat the process until no more non-spurious counterexample with the observation  $o$  is found, at which point Equation 25 becomes unsatisfiable.

To explore a different equivalence class of observation than that of observation  $o$ , CACHEFIX simply negates the verification goal. For timing-based attacks, as an example, the verification goal is changed as follows:

$$\Psi \wedge \neg \left( \left( \sum_{i=1}^N \text{miss}_i \right) = o \right) \quad (26)$$

We note that Equation 26 is satisfiable if and only if there exists an execution trace with observation differing from  $o$ .

**Runtime actions to improve side-channel freedom.** Our checker maintains the record of all explored observations and the symbolic conditions capturing the equivalence classes of respective observations. At each round of patch (i.e. runtime action) synthesis, we walk through this record and compute the necessary runtime actions for improving cache side-channel freedom.

**$\mathcal{O}_{\text{time}}$ .** Assume  $\Omega = \{\langle v_1, o_1 \rangle, \langle v_2, o_2 \rangle, \dots, \langle v_k, o_k \rangle\}$  where each  $o_i$  captures a unique number of observed cache misses and  $v_i$  symbolically captures all inputs that lead to observation  $o_i$ . Our goal is to manipulate executions so that they lead to the same number of cache misses. To this end, the patch synthesis stage determines the amount of cache misses that needs to be added for each element in  $\Omega$ . Concretely, the set of runtime actions generated are as follows:

$$\left\langle v_1, \left( \max_{i \in [1, k]} o_i - o_1 \right) \right\rangle, \dots, \left\langle v_k, \left( \max_{i \in [1, k]} o_i - o_k \right) \right\rangle \quad (27)$$

In practice, when a program is run with input  $I$ , we check whether  $I \in v_x$  for some  $x \in [1, k]$ . Subsequently,  $(\max_{i \in [1, k]} o_i - o_x)$  cache misses were injected before the program starts executing.

**$O_{\text{trace}}$ .** During trace-based attacks, the attacker makes an observation on the sequence of cache hits and misses in an execution trace. Therefore, our goal is to manipulate executions in such a fashion that all execution traces lead to the same sequence of cache hits and misses. To accomplish this, each runtime action involves the injection of cache misses or hits before execution, after execution or at an arbitrary point of execution. It also involves invalidating an address in cache. Concretely, this is formalized as follows:

$$\langle v_i, \langle (c_1, a_1), (c_2, a_2), \dots, (c_k, a_k) \rangle \rangle \quad (28)$$

where  $v_i$  captures the symbolic input condition where the runtime actions are employed. For any input satisfying  $v_i$ , we count the number of instructions executed. If the number of executed instructions reaches  $c_j$ , then we perform the action  $a_j$  (e.g. injecting hits/misses or invalidating an address in cache), for any  $j \in [1, k]$ .

As an example, consider a trace-based attack in the example of Figure 1(b). Our checker will manipulate counterexample traces by injecting cache misses and hits as follows (injected cache hits and misses are highlighted in bold):

$$\begin{aligned} tr_1'' &\equiv \langle \text{miss}, \text{miss}, \text{miss}, \text{hit}, \text{hit} \rangle \\ tr_2'' &\equiv \langle \text{miss}, \text{miss}, \text{miss}, \text{hit}, \text{hit} \rangle \end{aligned}$$

Therefore, the following actions are generated to ensure cache side-channel freedom against trace-based attacks:

$$\langle key = 255, \langle (0, \text{miss}) \rangle \rangle, \langle 0 \leq key \leq 254, \langle (4, \text{hit}) \rangle \rangle$$

We use standard string alignment algorithm [6] to make two traces equivalent (via insertion of cache hits/misses or substitution of hits to misses).

**Practical consideration.** In practice, the injection of a cache miss can be performed via accessing a fresh array element (cf. Figure 1(d)). However, if such injection does not happen to be in the beginning or at the end of execution, then the cache needs to be disabled. This is to ensure that the cache state remains unaffected even after the injection of an additional cache miss. Once the injection of cache miss is performed, the cache can be enabled. In ARM-based processor, a cache can be disabled and enabled via manipulating the C bit of CP15 system control register. The injection of a cache hit can be performed via tracking the last accessed memory address and re-accessing the same address.

Finally, the action to change a cache hit into a cache miss involves cache invalidation. Concretely, the memory address that was accessed via the respective instruction, needs to be invalidated in the cache. Through our checker, we symbolically track the memory address accessed at each memory-related instruction. When the program is run with input  $I \in v_i$ , we concretize all memory addresses with respect to  $I$ . Hence, while applying an action that involves cache invalidation, we know the exact memory address that needs to be invalidated. In ARM-based processor, the instruction MCR provides capabilities to invalidate a memory address in the cache.

We note the preceding manipulations on an execution requires additional registers. We believe this is possible by using some system register or using a locked portion in the cache.

**Properties guaranteed by CacheFix.** CACHEFIX satisfies the following crucial properties (details of proofs are included in the supplement [7]).

**PROPERTY 1. (Monotonicity)** Consider a victim program  $\mathcal{P}$  with sensitive input  $\mathcal{K}$ . Given attack models  $O_{\text{time}}$  or  $O_{\text{trace}}$ , assume that the channel capacity to quantify the uncertainty of guessing  $\mathcal{K}$  is  $\mathcal{G}_{\text{cap}}^{\mathcal{P}}$ . CacheFix guarantees that  $\mathcal{G}_{\text{cap}}^{\mathcal{P}}$  monotonically decreases with each synthesized patch (cf. Equation 27-28) employed at runtime.

**PROPERTY 2. (Convergence)** Let us assume a victim program  $\mathcal{P}$  with sensitive input  $\mathcal{K}$ . In the absence of any attacker, assume that the uncertainty to guess  $\mathcal{K}$  is  $\mathcal{G}_{\text{cap}}^{\text{init}}$ ,  $\mathcal{G}_{\text{shn}}^{\text{init}}$  and  $\mathcal{G}_{\text{min}}^{\text{init}}$ , via channel capacity, Shannon entropy and Min entropy, respectively. If our checker terminates and all synthesized patches are applied at runtime, then our framework guarantees that the channel capacity (respectively, Shannon entropy and Min entropy) will remain  $\mathcal{G}_{\text{cap}}^{\text{init}}$  (respectively,  $\mathcal{G}_{\text{shn}}^{\text{init}}$  and  $\mathcal{G}_{\text{min}}^{\text{init}}$ ) even in the presence of attacks captured via  $O_{\text{time}}$  and  $O_{\text{trace}}$ .

## 6 IMPLEMENTATION AND EVALUATION

**Implementation setup.** The input to CACHEFIX is the target program and a cache configuration. We have implemented CACHEFIX on top of CBMC model checker [1]. CBMC is a bounded model checker that first builds a formula representation of the input program via symbolic execution. Subsequently, it checks the (un)satisfiability of this formula against a specification property. The implementation of our checker impacts the entire workflow of CBMC. We first modify the symbolic execution engine of CBMC to insert the predicates related to cache semantics. As a result, upon the termination of symbolic execution, the formula representation of the program encodes both the cache semantics and the program semantics. Secondly, we systematically rewrite this formula based on our abstraction refinement, with the aim of verifying cache side-channel freedom. Finally, we modify the verification engine of CBMC to systematically explore different counterexamples, instrument patches and refining the side-channel freedom properties *on-the-fly*. To manipulate and solve symbolic formulas, we leverage Z3 theorem prover. All reported experiments were performed on an Intel I7 machine, having 8GB RAM and running OSX.

**Subject programs.** We have chosen subjects from OpenSSL [5], GDK [3], libfixedtimefixedpoint [4] and elliptic curve routines from FourQlib [2] libraries to evaluate CACHEFIX. The choice of our subjects is driven by the criticality of the respective routines in developing cryptographic software. To stress test our checker, we include representative routines exhibiting constant cache-timing, as well as routines exhibiting variable cache timing. Some salient features of our chosen subjects appear in Table 1.

**Efficiency of checking.** Table 1 captures a summary of our evaluation for CACHEFIX. For all experiments in Table 1, we configured the cache to be direct-mapped, with a total size of 1 KB and a line size of 32 bytes. The outcome of this evaluation is either a successful verification (✓) or a non-spurious counterexample (✗). As observed from Table 1, CACHEFIX was able to accomplish the verification tasks for all subjects only within a few minutes. The maximum time taken by our checker was 390 seconds for the routine `fix_pow` – a constant time implementation of powers ( $x^y$ ). `fix_pow` has



**Table 1: Summary of CACHEFIX Evaluation**

| Library     | Routine         | Size (LOC) | $O_{time}$ |             | $O_{trace}$ |             |
|-------------|-----------------|------------|------------|-------------|-------------|-------------|
|             |                 |            | Result     | Time (secs) | Result      | Time (secs) |
| OpenSSL [5] | AES128          | 740        | ✗          | 148.73      | ✗           | 175.34      |
|             | DES             | 2124       | ✗          | 105.87      | ✗           | 110.32      |
|             | RC5             | 1613       | ✓          | 26.88       | ✓           | 34.84       |
| GDK [3]     | keyname         | 712        | ✗          | 21.75       | ✗           | 24.32       |
|             | unicode         | 862        | ✗          | 27.49       | ✗           | 32.09       |
| fixedt [4]  | fix_eq          | 334        | ✓          | 1.70        | ✓           | 4.31        |
|             | fix_cmp         | 400        | ✓          | 2.09        | ✓           | 2.08        |
|             | fix_mul         | 930        | ✓          | 22.44       | ✓           | 20.19       |
|             | fix_conv_64     | 350        | ✓          | 1.69        | ✓           | 1.78        |
|             | fix_sqrt        | 2480       | ✓          | 60.54       | ✓           | 67.90       |
|             | fix_exp         | 1128       | ✓          | 53.47       | ✓           | 55.12       |
|             | fix_ln          | 1140       | ✓          | 58.89       | ✓           | 61.11       |
|             | fix_pow         | 2890       | ✓          | 389.97      | ✓           | 377.55      |
|             | fix_ceil        | 390        | ✓          | 1.70        | ✓           | 4.65        |
|             | fix_conv_double | 650        | ✓          | 2.70        | ✓           | 4.16        |
| FourQ [2]   | fix_frac        | 370        | ✗          | 22.14       | ✗           | 22.15       |
|             | eccmadd         | 1550       | ✓          | 220.59      | ✓           | 214.16      |
|             | eccnorm         | 1303       | ✓          | 105.97      | ✓           | 114.93      |
|             | pt_setup        | 1345       | ✓          | 10.45       | ✓           | 14.90       |
|             | eccdouble       | 1364       | ✓          | 285.70      | ✓           | 312.31      |
|             | R1_to_R2        | 1352       | ✓          | 73.07       | ✓           | 84.11       |
|             | R1_to_R3        | 1328       | ✓          | 26.95       | ✓           | 24.89       |
|             | R2_to_R4        | 1322       | ✓          | 32.29       | ✓           | 31.12       |
|             | R5_to_R1        | 1387       | ✓          | 22.07       | ✓           | 24.32       |
|             | eccpt_validate  | 1406       | ✗          | 34.48       | ✗           | 34.31       |

complex memory access patterns, however, its flat structure ensures cache side-channel freedom.

Both AES and DES are single path programs. However, due to the input-dependent memory accesses, they are not cache side-channel free. To this end, CACHEFIX generated counterexample traces within 2-3 minutes. In contrast to AES and DES, RC5 does not exhibit input-dependent memory accesses. As a result, our checker established the proof of cache side-channel freedom within just 1 minute.

The routines used from GDK library employ a binary search on a large table. This is to discover, for instance, the unicode from the `ascii` value of a keystroke. Since the number of iterations in the binary search is highly dependent on the search input (in this case, a keystroke), the search operation will likely to exhibit diverse cache behaviour for different search inputs. CACHEFIX generated relevant counterexamples within a minute to prove the existence of cache side-channel in the GDK library. Finally, both `libfixedtimefixedpoint` [4] and `FourQlib` [2] contain routines that *are not cache side-channel free*. This includes routines `fix_frac` and `ecc_point_validate` (cf. validate in Table 1). The side-channel exists due to input-dependent loop trip counts. CACHEFIX detected these side-channels within half a minute. We note that the respective libraries have included developer comments involving the security risks in both `fix_frac` and `ecc_point_validate`.

CacheFix verifies or generates real counterexamples at an average within 70.38 secs w.r.t. attack model  $O_{time}$  and at an average within 74.12 secs w.r.t.  $O_{trace}$ .

**Table 2: Overhead from monitors**

| Routine        | $O_{time}$         |             | $O_{trace}$        |             |
|----------------|--------------------|-------------|--------------------|-------------|
|                | #Equivalence class | Time (secs) | #Equivalence class | Time (secs) |
| AES128         | 3                  | 5           | 38                 | 1271        |
| DES            | 333                | 444         | 982                | 12601       |
| fix_frac       | 82                 | 521         | 82                 | 956         |
| eccpt_validate | 20                 | 22          | 20                 | 234         |
| keyname        | 41                 | 1119        | 41                 | 1324        |
| unicode        | 43                 | 197         | 43                 | 229         |

**Overhead from monitors.** We evaluated the overhead due to counterexample exploration and patch generation (cf. Section 5). For the reported experiments, we configured a direct-mapped 1 KB cache with 32 bytes cache line (detailed experiments with a variety of LRU and FIFO cache configurations are included in the supplement [7]). Table 2 outlines a summary of our findings.

Except AES and DES, other subject routines involve multiple program paths, which, in turn exhibit diverse cache behaviours. For such routines, the cache behaviour of a single program path is independent of program inputs and the variability in cache behaviour appears due to different counterexamples exhibiting different program paths. As observed from Table 2, for a given subject routine chosen from these libraries, approximately the same number of equivalence classes were explored for both attack models. Each explored equivalence class was primarily attributed to a unique program path. Nevertheless, the overhead of CACHEFIX in attack model  $O_{trace}$  is higher than the overhead in attack model  $O_{time}$ . This is due to more computations in the patching process for  $O_{trace}$  (cf. Section 5), as compared to the patching process for  $O_{time}$ .

Both AES and DES exhibit diverse cache behaviour due to input-dependent memory accesses. As observed from Table 2, CACHEFIX discovers significantly more equivalence classes w.r.t. attack model  $O_{trace}$  as compared to the number of equivalence classes w.r.t. attack model  $O_{time}$ . This implies AES is more vulnerable to  $O_{trace}$  as compared to  $O_{time}$ . Excluding DES subject to  $O_{trace}$ , our exploration terminates in all scenarios within 20 mins. For DES, CacheFix terminates in 3.5 hours after exploring 982 equivalence classes w.r.t.  $O_{trace}$ .

The overhead due to counterexample exploration and patching is 2.27x more w.r.t. attack model  $O_{trace}$ , as compared to the overhead w.r.t.  $O_{time}$ . Moreover, excluding DES, CacheFix explores all equivalence classes of observations within 20 minutes in all scenarios.

## 7 REVIEW OF PRIOR WORKS

Earlier works on cache analysis are based on abstract interpretation [35] and its combination with model checking [18], to estimate the worst-case execution time (WCET) of a program. In contrast to these approaches, CACHEFIX automatically builds and refine the abstraction of cache semantics for verifying side-channel freedom.

Cache attacks are one of the most critical side-channel attacks [8, 14, 25–28, 32, 37, 38]. In contrast to the literature on side-channel attacks, we do not aim to engineer new cache attacks in this paper. Based on a configurable attack model, CACHEFIX verifies and reinstates the cache side-channel freedom of arbitrary programs.

CACHEFIX is orthogonal to approaches proposing countermeasures for thwarting side-channel attacks [21, 36]. With our CACHEFIX approach, we show that it is possible to leverage the verification results and automatically generate patches to improve and even completely eliminate the cache side channels in a program. Moreover, CACHEFIX approach can be leveraged to formally verify whether existing countermeasures are capable to ensure side-channel freedom.

In contrast to recent approaches on statically analyzing cache side channels [15, 22, 29, 30], our CACHEFIX approach automatically constructs and refines the abstractions for verifying cache

side-channel freedom. Moreover, approaches based on static analysis are not directly applicable to explore all equivalence classes of observations by an attacker and subsequently, generate patches to be employed at runtime. Our proposed approach serves the dual purpose of verification and runtime monitoring to ensure cache side-channel freedom of a program. CACHEFIX targets verification of arbitrary software programs, over and above constant-time implementations [9, 12]. Existing works based on symbolic execution [11, 34], taint analysis [20, 33] and verifying timing-channel freedom [10] ignore cache attacks. Moreover, these works do not provide capabilities for automatic abstraction refinement and patch synthesis for ensuring side-channel freedom. Finally, in contrast to these works, we show that our CACHEFIX approach scales with routines from real cryptographic libraries.

Finally, recent approaches on testing and quantifying cache side-channel leakage [13, 16, 17] are complementary approaches. These works aim to test (in contrast to verification) the cache side-channel vulnerabilities of a program and they do not provide capabilities to ensure cache side-channel freedom.

## 8 DISCUSSION

In this paper, we propose CACHEFIX, a novel approach to automatically verify and restore cache side-channel freedom of arbitrary programs. The key novelty in our approach is two fold. Firstly, our CACHEFIX approach automatically builds and refines abstraction of cache semantics. Although targeted to verify cache side-channel freedom, we believe CACHEFIX is applicable to verify other cache timing properties, such as WCET. Secondly, the core symbolic engine of CACHEFIX systematically combines its reasoning power with runtime monitoring to ensure cache side-channel freedom during program execution. Our evaluation reveals promising results, for 25 routines from several cryptographic libraries, CACHEFIX (dis)proves cache side-channel freedom within an average 75 seconds. Moreover, in most scenarios, CACHEFIX generated patches within 20 minutes to ensure cache side-channel freedom during program execution. Despite this result, we believe that CACHEFIX is only an initial step for the automated verification of cache side-channel freedom. In particular, we do not account cache attacks that are more powerful than timing or trace-based attacks. Besides, we do not implement the synthesized patches in a commodity embedded system to check their performance impact. We hope that the community will take this effort forward and push the adoption of formal tools for the evaluation of cache side-channel. For reproducibility and research, our tool and all experimental data are publicly available: **(blinded)**

## REFERENCES

- [1] [n. d.]. CBMC: Bounded Model Checking for Software. ([n. d.]). <http://www.cprover.org/cbmc/> (Date last accessed 23-October-2017).
- [2] [n. d.]. FourQLib Library. ([n. d.]). <https://github.com/Microsoft/FourQlib/> (Date last accessed 20-October-2017).
- [3] [n. d.]. GDK Library. ([n. d.]). <https://developer.gnome.org/gdk3/3.22/> (Date last accessed 20-October-2017).
- [4] [n. d.]. A library for doing constant-time fixed-point numeric operations. ([n. d.]). <https://github.com/kmowery/libfixedtimefixedpoint/> (Date last accessed 20-October-2017).
- [5] [n. d.]. OpenSSL Library. ([n. d.]). <https://github.com/openssl/openssl/> (Date last accessed 20-October-2017).
- [6] [n. d.]. SSW Library. ([n. d.]). <https://github.com/mengyao/Complete-Striped-Smith-Waterman-Library> (Date last accessed 23-October-2017).
- [7] [n. d.]. Symbolic Verification of Cache Side-channel Freedom. ([n. d.]). [https://github.com/esweek2018/emsoft2018/blob/master/cache\\_fix\\_supplement.pdf](https://github.com/esweek2018/emsoft2018/blob/master/cache_fix_supplement.pdf).
- [8] Onur Acıçmez and Çetin Kaya Koç. 2006. Trace-driven cache attacks on AES. In *Information and Communications Security*. Springer.
- [9] José Bacerlar Almeida, Manuel Barbosa, Gilles Barthe, François Dupressoir, and Michael Emmi. 2016. Verifying Constant-Time Implementations. In *USENIX*. 53–70.
- [10] Timos Antonopoulos, Paul Gazzillo, Michael Hicks, Eric Koskinen, Tachio Terauchi, and Shiyi Wei. 2017. Decomposition instead of self-composition for proving the absence of timing channels. In *PLDI*. 362–375.
- [11] Michael Backes, Boris Köpf, and Andrey Rybalchenko. 2009. Automatic Discovery and Quantification of Information Leaks. In *IEEE S&P*. 141–153.
- [12] Gilles Barthe, Gustavo Betarte, Juan Diego Campo, Carlos Daniel Luna, and David Pichardie. 2014. System-level Non-interference for Constant-time Cryptography. In *CCS*. 1267–1279.
- [13] Tiyash Basu and Sudipta Chattopadhyay. 2017. Testing Cache Side-Channel Leakage. In *ICST Workshops*. 51–60.
- [14] Daniel J Bernstein. 2005. Cache-timing attacks on AES. (2005).
- [15] Pablo Cañones, Boris Köpf, and Jan Reineke. 2017. Security Analysis of Cache Replacement Policies. In *POST*. 189–209.
- [16] Sudipta Chattopadhyay. 2017. Directed Automated Memory Performance Testing. In *TACAS*. 38–55.
- [17] Sudipta Chattopadhyay, Moritz Beck, Ahmed Rezine, and Andreas Zeller. 2017. Quantifying the information leak in cache attacks via symbolic execution. In *MEMOCODE*. 25–35.
- [18] Sudipta Chattopadhyay and Abhik Roychoudhury. 2013. Scalable and precise refinement of cache timing analysis via path-sensitive verification. *Real-Time Systems* 49, 4 (2013), 517–562.
- [19] Edmund M. Clarke, Armin Biere, Richard Raimi, and Yunshan Zhu. 2001. Bounded Model Checking Using Satisfiability Solving. *Formal Methods in System Design* 19, 1 (2001), 7–34.
- [20] James Clause, Wanchun Li, and Alessandro Orso. 2007. Dytan: a generic dynamic taint analysis framework. In *ISSTA*. 196–206.
- [21] Stephen Crane, Andrei Homescu, Stefan Brunthaler, Per Larsen, and Michael Franz. 2015. Thwarting Cache Side-Channel Attacks Through Dynamic Software Diversity. In *NDSS*.
- [22] Goran Doychev, Boris Köpf, Laurent Mauborgne, and Jan Reineke. 2015. CacheAudit: a tool for the static analysis of cache side channels. *TISSEC* 18, 1 (2015), 4.
- [23] Moritz Lipp et al. 2018. Meltdown. *ArXiv e-prints* (2018). arXiv:1801.01207
- [24] Paul Kocher et al. 2018. Spectre Attacks: Exploiting Speculative Execution. *ArXiv e-prints* (2018). arXiv:1801.01203
- [25] Qian Ge, Yuval Yarom, David Cock, and Gernot Heiser. 2016. A Survey of Microarchitectural Timing Attacks and Countermeasures on Contemporary Hardware. In *Cryptology ePrint Archive*. <https://eprint.iacr.org/2016/613.pdf/>.
- [26] Daniel Gruss, Raphael Spreitzer, and Stefan Mangard. 2015. Cache Template Attacks: Automating Attacks on Inclusive Last-Level Caches. In *USENIX Security*.
- [27] Roberto Guanciale, Hamed Nemati, Christoph Baumann, and Mads Dam. 2016. Cache Storage Channels: Alias-Driven Attacks and Verified Countermeasures. In *IEEE Symposium on Security and Privacy*. 38–55.
- [28] David Gullasch, Endre Bangerter, and Stephan Krenn. 2011. Cache games—bringing access-based cache attacks on AES to practice. In *IEEE Symposium on Security and Privacy*. IEEE.
- [29] Boris Köpf and David A. Basin. 2007. An information-theoretic model for adaptive side-channel attacks. In *CCS*. 286–296.
- [30] Boris Köpf, Laurent Mauborgne, and Martín Ochoa. 2012. Automatic quantification of cache side-channels. In *CAV*. Springer.
- [31] Moritz Lipp, Daniel Gruss, Raphael Spreitzer, Clémentine Maurice, and Stefan Mangard. 2016. ARMageddon: Cache Attacks on Mobile Devices. In *USENIX Security Symposium*. 549–564.
- [32] Fangfei Liu, Yuval Yarom, Qian Ge, Gernot Heiser, and Ruby B. Lee. 2015. Last-Level Cache Side-Channel Attacks are Practical. In *IEEE Symposium on Security and Privacy*. 605–622.
- [33] James Newsome, Stephen McCamant, and Dawn Song. 2009. Measuring channel capacity to distinguish undue influence. In *PLAS*. 73–85.
- [34] Corina S. Pasareanu, Quoc-Sang Phan, and Pasquale Malacaria. 2016. Multi-run side-channel analysis using Symbolic Execution and Max-SMT. In *CSF*.
- [35] Henrik Theiling, Christian Ferdinand, and Reinhard Wilhelm. 2000. Fast and precise WCET prediction by separated cache and path analyses. *Real-Time Systems* 18, 2-3 (2000).
- [36] Zhenghong Wang and Ruby B. Lee. 2007. New Cache Designs for Thwarting Software Cache-based Side Channel Attacks. In *ISCA*. 494–505.
- [37] Yuval Yarom and Katrina Falkner. 2014. FLUSH+RELOAD: A High Resolution, Low Noise, L3 Cache Side-Channel Attack. In *USENIX Security Symposium*. 719–732.
- [38] Yuval Yarom, Daniel Genkin, and Nadia Heninger. 2017. CacheBleed: a timing attack on OpenSSL constant-time RSA. *J. Cryptographic Engineering* 7, 2 (2017), 99–112.

## APPENDIX

The appendix includes additional cache models (e.g. LRU and FIFO) incorporated within CACHEFIX, the theoretical guarantees and additional experimental results.

### Theoretical Guarantees

In this section, we include the detailed proof of the properties satisfied by CACHEFIX.

**PROPERTY 3. (Monotonicity)** Consider a victim program  $\mathcal{P}$  with sensitive input  $\mathcal{K}$ . Given attack models  $O_{time}$  or  $O_{trace}$ , assume that the channel capacity to quantify the uncertainty of guessing  $\mathcal{K}$  is  $\mathcal{G}_{cap}^{\mathcal{P}}$ . CacheFix guarantees that  $\mathcal{G}_{cap}^{\mathcal{P}}$  monotonically decreases with each synthesized patch (cf. Equation 27-28) employed at runtime.

**PROOF.** Consider the generic attack model  $O : \{h, m\}^* \rightarrow \mathbb{X}$  that maps each trace to an element in the countable set  $\mathbb{X}$ . For a victim program  $\mathcal{P}$ , assume  $TR \subseteq \{h, m\}^*$  is the set of all execution traces. After one round of patch synthesis, assume  $TR' \subseteq \{h, m\}^*$  is the set of all execution traces in  $\mathcal{P}$  when the synthesized patches are applied at runtime. By construction, each round of patch synthesis merges two equivalence classes of observations (cf. Algorithm 3), hence, making them indistinguishable by the attacker  $O$ . As a result, the following relationship holds:

$$|O(TR)| = |O(TR')| + 1 \quad (29)$$

Channel capacity  $\mathcal{G}_{cap}^{\mathcal{P}}$  equals to  $\log |O(TR)|$  for the original program  $\mathcal{P}$ , but it reduces to  $\log |O(TR')|$  when the synthesized patches are applied. We conclude the proof as the same argument holds for any round of patch synthesis.  $\square$

**PROPERTY 4. (Convergence)** Let us assume a victim program  $\mathcal{P}$  with sensitive input  $\mathcal{K}$ . In the absence of any attacker, assume that the uncertainty to guess  $\mathcal{K}$  is  $\mathcal{G}_{cap}^{init}$ ,  $\mathcal{G}_{shn}^{init}$  and  $\mathcal{G}_{min}^{init}$ , via channel capacity, Shannon entropy and Min entropy, respectively. If our checker terminates and all synthesized patches are applied at runtime, then our framework guarantees that the channel capacity (respectively, Shannon entropy and Min entropy) will remain  $\mathcal{G}_{cap}^{init}$  (respectively,  $\mathcal{G}_{shn}^{init}$  and  $\mathcal{G}_{min}^{init}$ ) even in the presence of attacks captured via  $O_{time}$  and  $O_{trace}$ .

**PROOF.** Consider the generic attack model  $O : \{h, m\}^* \rightarrow \mathbb{X}$ , mapping each execution trace to an element in the countable set  $\mathbb{X}$ . We assume a victim program  $\mathcal{P}$  that exhibits a set of execution traces  $TR \subseteq \{h, m\}^*$ . From Equation 29, we know that  $|O(TR)|$  decreases with each round of patch synthesis. Given that our checker terminates, we obtain the program  $\mathcal{P}$ , together with a set of synthesized patches that are applied when  $\mathcal{P}$  executes. Assume  $TR^f \in \{h, m\}^*$  is the set of execution traces obtained from  $\mathcal{P}$  when all patches are systematically applied. Clearly,  $|O(TR^f)| = 1$ .

The channel capacity of  $\mathcal{P}$ , upon the termination of our checker, is  $\log(|O(TR^f)|) = \log 1 = 0$ . This concludes that the channel capacity does not change even in the presence of attacks  $O_{time}$  and  $O_{trace}$ .

For a given distribution  $\lambda$  of sensitive input  $\mathcal{K}$ , Shannon entropy  $\mathcal{G}_{shn}^{init}$  is computed as follows:

$$\mathcal{G}_{shn}^{init}(\lambda) = - \sum_{\mathcal{K} \in \mathbb{K}} \lambda(\mathcal{K}) \log_2 \lambda(\mathcal{K}) \quad (30)$$

where  $\mathbb{K}$  captures the domain of sensitive input  $\mathcal{K}$ . For a given equivalence class of observation  $o \in O(TR^f)$ , the remaining uncertainty is computed as follows:

$$\mathcal{G}_{shn}^{final}(\lambda_o) = - \sum_{\mathcal{K} \in \mathbb{K}} \lambda_o(\mathcal{K}) \log_2 \lambda_o(\mathcal{K}) \quad (31)$$

$\lambda_o(\mathcal{K})$  captures the probability that the sensitive input is  $\mathcal{K}$ , given the observation  $o$  is made by the attacker. Finally, to evaluate the remaining uncertainty of the patched program version,  $\mathcal{G}_{shn}^{final}(\lambda_o)$  is averaged over all equivalence class of observations as follows:

$$\mathcal{G}_{shn}^{final}(\lambda_{O(TR^f)}) = \sum_{o \in O(TR^f)} pr(o) \mathcal{G}_{shn}^{final}(\lambda_o) \quad (32)$$

where  $pr(o)$  captures the probability of the observation  $o \in O(TR^f)$ . However, we have  $|O(TR^f)| = 1$ . Hence, for any  $o \in O(TR^f)$ , we get  $pr(o) = 1$  and  $\lambda_o(\mathcal{K}) = \lambda(\mathcal{K})$ . Plugging these observations into Equation 32 and Equation 31, we get the following:

$$\begin{aligned} \mathcal{G}_{shn}^{final}(\lambda_{O(TR^f)}) &= \sum_{o \in O(TR^f)} \mathcal{G}_{shn}^{final}(\lambda_o) \\ &= - \sum_{\mathcal{K} \in \mathbb{K}} \lambda(\mathcal{K}) \log_2 \lambda(\mathcal{K}) \\ &= \mathcal{G}_{shn}^{init}(\lambda) \end{aligned} \quad (33)$$

Finally, for a given distribution  $\lambda$  of sensitive input  $\mathcal{K}$ , the min entropy  $\mathcal{G}_{min}^{init}$  is computed as follows:

$$\mathcal{G}_{min}^{init}(\lambda) = -\log_2 \max_{\mathcal{K} \in \mathbb{K}} \lambda(\mathcal{K}) \quad (34)$$

Therefore, min entropy captures the best strategy of an attacker, that is, to choose the most probable secret.

Similar to Shannon entropy, for a given equivalence class of observation  $o \in O(TR^f)$ , the remaining uncertainty is computed as follows:

$$\mathcal{G}_{min}^{init}(\lambda_o) = -\log_2 \max_{\mathcal{K} \in \mathbb{K}} \lambda_o(\mathcal{K}) \quad (35)$$

$\lambda_o(\mathcal{K})$  captures the probability that the sensitive input is  $\mathcal{K}$ , given the observation  $o$  is made by the attacker.

Finally, we obtain the min entropy of the patched program version via the following relation:

$$\mathcal{G}_{min}^{final}(\lambda_{O(TR^f)}) = -\log_2 \sum_{o \in O(TR^f)} pr(o) \max_{\mathcal{K} \in \mathbb{K}} \lambda_o(\mathcal{K}) \quad (36)$$

Since  $pr(o) = 1$  and  $\lambda_o(\mathcal{K}) = \lambda(\mathcal{K})$  for any  $o \in O(TR^f)$ , we get the following from Equation 36 and Equation 35:

$$\begin{aligned} \mathcal{G}_{min}^{final}(\lambda_{O(TR^f)}) &= -\log_2 \sum_{o \in O(TR^f)} \max_{\mathcal{K} \in \mathbb{K}} \lambda_o(\mathcal{K}) \\ &= -\log_2 \max_{\mathcal{K} \in \mathbb{K}} \lambda(\mathcal{K}) \\ &= \mathcal{G}_{min}^{init}(\lambda) \end{aligned} \quad (37)$$

Equation 33 and Equation 37 conclude this proof.  $\square$

## Modeling LRU and FIFO cache semantics

To formulate the conditions for conflict misses in set-associative caches, it is necessary to understand the notion of cache conflict. We use the following definition of cache conflict to formulate  $\Gamma(r_i)$ :

**DEFINITION 1. (Cache conflict)**  $r_j$  generates a cache conflict to  $r_i$  if and only if  $1 \leq j < i$ ,  $\sigma(r_j) \neq \sigma(r_i)$  and the execution of  $r_j$  can change the relative position of  $\sigma(r_i)$  within the  $set(r_i)$ -state immediately before instruction  $r_i$ .

Recall that  $\sigma(r_i)$  captures the memory block accessed at  $r_i$  and  $set(r_i)$  captures the cache set accessed by  $r_i$ . The state of a cache set is an ordered  $\mathcal{A}$ -tuple – capturing the relative positions of all memory blocks within the respective cache set. For instance,  $\langle m_1, m_2 \rangle$  captures the state of a two-associative cache set. The rightmost memory block (*i.e.*  $m_2$ ) captures the first memory block to be evicted from the cache set if a block  $m \notin \{m_1, m_2\}$  is accessed and mapped to the same cache set.

**Challenges with LRU policy.** To illustrate the unique challenges related to set-associative caches, let us consider the following sequence of memory accesses in a two-way associative cache and with LRU replacement policy:  $(r_1 : m_1) \rightarrow (r_2 : m_2) \rightarrow (r_3 : m_2) \rightarrow (r_4 : m_1)$ . We assume both  $m_1$  and  $m_2$  are mapped to the same cache set. If the cache is empty before  $r_1$ ,  $r_4$  will still incur a *cache hit*. This is because,  $r_4$  suffers cache conflict only once, from the memory block  $m_2$ . To incorporate the aforementioned phenomenon into our cache semantics, we only count cache conflicts from the closest access to a given memory block. Therefore, in our example, we count cache conflicts to  $r_4$  from  $r_3$  and discard the cache conflict from  $r_2$ . Formally, we introduce the following additional condition for instruction  $r_j$  to inflict a cache conflict to instruction  $r_i$ .

$\phi_{ji}^{eqv,lru}$  : No instruction between  $r_j$  and  $r_i$  accesses the same memory block as  $r_j$ . This is to ensure that  $r_j$  is the closest to  $r_i$  in terms of accessing the memory block  $\sigma(r_j)$ . We capture  $\phi_{ji}^{eqv,lru}$  formally as follows:

$$\phi_{ji}^{eqv,lru} \equiv \bigwedge_{j < k < i} (\rho_{jk}^{tag} \vee \neg \rho_{jk}^{set} \vee \neg guard_k) \quad (38)$$

Hence,  $r_j$  inflicts a unique cache conflict to  $r_i$  only if  $\phi_{ji}^{eqv,lru}$ ,  $\phi_{ji}^{cnf,lru} \equiv \phi_{ji}^{cnf,dir}$ ,  $\phi_{ji}^{rel,lru} \equiv \phi_{ji}^{rel,dir}$  are all satisfiable.

**Challenges with FIFO policy.** Unlike LRU replacement policy, the cache state does not change for a cache hit in FIFO replacement policy. For example, consider the following sequence of memory accesses in a two-way associative FIFO cache:  $(r_1 : m_1) \rightarrow (r_2 : m_2) \rightarrow (r_3 : m_1) \rightarrow (r_4 : m_1)$ . Let us assume  $m_1, m_2$  map to the same cache set and the cache is empty before  $r_1$ . In this example,  $r_2$  generates a cache conflict to  $r_4$  even though  $m_1$  is accessed between  $r_2$  and  $r_4$ . This is because  $r_3$  is a cache hit and it does not change cache states.

In general, to formulate  $\Gamma(r_i)$ , we need to know whether any instruction  $r_j$ , prior to  $r_i$ , was a cache miss. This, in turn, is captured via  $\Gamma(r_j)$ . Concretely,  $r_j$  generates a unique cache conflict to  $r_i$  if all the following conditions are satisfied.

$\phi_{ji}^{cnf,fifo}$  : If  $r_j$  accesses the same cache set as  $r_i$ , but accesses a different cache-tag as compared to  $r_i$  and  $r_j$  suffers a cache miss.

This is formalized as follows:

$$\phi_{ji}^{cnf,fifo} \equiv \rho_{ji}^{tag} \wedge \rho_{ji}^{set} \wedge \Gamma(r_j) \quad (39)$$

$\phi_{ji}^{rel,fifo}$  : No cache miss between  $r_j$  and  $r_i$  access the same memory block as  $r_i$ .  $\phi_{ji}^{rel,fifo}$  ensures that the relative position of the memory block  $\sigma(r_i)$  within  $set(r_i)$  was not reset between  $r_j$  and  $r_i$ .  $\phi_{ji}^{rel,fifo}$  is formalized as follows:

$$\phi_{ji}^{rel,fifo} \equiv \bigwedge_{j < k < i} (\rho_{ki}^{tag} \vee \neg \rho_{ki}^{set} \vee \neg guard_k \vee \neg \Gamma(r_k)) \quad (40)$$

$\phi_{ji}^{eqv,fifo}$  : No cache miss between  $r_j$  and  $r_i$  access the same memory block as  $r_j$ . We note that  $\phi_{ji}^{eqv,fifo}$  ensures that  $r_j$  is the closest cache miss to  $r_i$  accessing the memory block  $\sigma(r_j)$ . This, in turn, ensures that we count the cache conflict from memory block  $\sigma(r_j)$  to instruction  $r_i$  only once. We formulate  $\phi_{ji}^{eqv,fifo}$  as follows:

$$\phi_{ji}^{eqv,fifo} \equiv \bigwedge_{j < k < i} (\rho_{jk}^{tag} \vee \neg \rho_{jk}^{set} \vee \neg guard_k \vee \neg \Gamma(r_k)) \quad (41)$$

### Formulating cache conflict in set-associative caches.

With the intuition mentioned in the preceding paragraphs, we formalize the unique cache conflict from  $r_j$  to  $r_i$  via the following logical conditions:

$$\Theta_{j,i}^{+,x} \equiv (\phi_{ji}^{cnf,x} \wedge \phi_{ji}^{rel,x} \wedge \phi_{ji}^{eqv,x} \wedge guard_j) \Rightarrow (\eta_{ji} = 1) \quad (42)$$

$$\Theta_{j,i}^{-,x} \equiv (\neg \phi_{ji}^{cnf,x} \vee \neg \phi_{ji}^{rel,x} \vee \neg \phi_{ji}^{eqv,x} \vee \neg guard_j) \Rightarrow (\eta_{ji} = 0) \quad (43)$$

where  $x = \{lru, fifo\}$ . Concretely,  $\eta_{ji}$  is set to 1 if  $r_j$  creates a unique cache conflict to  $r_i$  and  $\eta_{ji}$  is set to 0 otherwise.

**Computing  $\Gamma(r_i)$  for Set-associative Caches.** To formulate  $\Gamma(r_i)$  for set-associative caches, we need to check whether the number of unique cache conflicts to  $r_i$  exceeds the associativity ( $\mathcal{A}$ ) of the cache. Based on this intuition, we formalize  $\Gamma(r_i)$  for set-associative caches as follows:

$$\Gamma(r_i) \equiv guard_i \wedge \left( \Theta_i^{cold} \vee \left( \left( \sum_{j \in [1,i)} \eta_{ji} \right) \geq \mathcal{A} \right) \right) \quad (44)$$

We note that  $\sum_{j \in [1,i)} \eta_{ji}$  accurately counts the number of unique cache conflicts to the instruction  $r_i$  (*cf.* Equation 42-Equation 43). Hence, the condition  $(\sum_{j \in [1,i)} \eta_{ji} \geq \mathcal{A})$  precisely captures whether  $\sigma(r_i)$  is replaced from the cache before  $r_i$  is executed. If  $r_i$  does not suffer a cold miss and  $(\sum_{j \in [1,i)} \eta_{ji} < \mathcal{A})$ , then  $r_i$  will be a cache hit when executed, as captured by the condition  $\neg \Gamma(r_i)$ .

## Detailed Runtime Monitoring

Algorithm 3 outlines the overall process. The procedure MONITORING takes the following inputs:

- $\Psi$ : A symbolic representation of program and cache semantics with the current level of abstraction,
- $\mathcal{O}$  and  $\varphi$ : The model of the attacker ( $\mathcal{O}$ ) and a property  $\varphi$  initially capturing cache side-channel freedom w.r.t.  $\mathcal{O}$ ,

---

**Algorithm 3** Monitor extraction and instrumentation

---

```
1: procedure MONITORING( $\Psi, O, \varphi, Pred, Pred_{cur}, \Gamma$ )
2:   /* If  $\varphi$  captures side-channel freedom, then  $trace$  is
3:   any of the two traces constituting the counterexample */
4:    $(res, trace) := \text{VERIFY}(\Psi, \varphi)$ 
5:   while  $(res = false) \wedge (trace \neq \text{spurious})$  do
6:     /* Extract observation from  $trace$  */
7:      $o := \text{GETOBSERVATION}(trace)$ 
8:     /* Extract monitor from  $trace$  */
9:      $v_o := v := \text{EXTRACTMONITOR}(trace)$ 
10:    /* Refine  $\Psi$  to find unique counterexamples */
11:     $\Psi := \Psi \wedge \neg v$ 
12:    /* Refine  $\varphi$  to find all traces exhibiting  $o$  */
13:     $\varphi := \text{REFINEOBJECTIVE}(\varphi, o)$ 
14:    /* Check the unsatisfiability of  $\Psi \wedge \neg \varphi$  */
15:     $(res', trace') := \text{VERIFY}(\Psi, \varphi)$ 
16:    while  $(res' = false)$  do
17:      if  $(trace' \neq \text{spurious})$  then
18:         $v := \text{EXTRACTMONITOR}(trace')$ 
19:        /* Combine monitors with observation  $o$  */
20:         $v_o := v_o \vee v$ 
21:        /* Refine  $\Psi$  for unique counterexamples */
22:         $\Psi := \Psi \wedge \neg v$ 
23:        /* Check the unsatisfiability of  $\Psi \wedge \neg \varphi$  */
24:         $(res', trace') := \text{VERIFY}(\Psi, \varphi)$ 
25:      else
26:        /* Refine abstraction to repeat verification */
27:         $\text{ABSREFINE}(\Psi, Pred, Pred_{cur}, trace', \Gamma)$ 
28:         $(res', trace') := \text{VERIFY}(\Psi, \varphi)$ 
29:      end if
30:    end while
31:    Let  $\Omega$  holds the set of monitor, observation pairs
32:     $\Omega \cup := \{(v_o, o)\}$ 
33:    /* Instrument patches for monitor  $v_o$  */
34:     $\text{INSTRUMENTPATCH}(\Omega, O)$ 
35:    /* Refine objective to find new observations */
36:     $\varphi := \neg \varphi$ 
37:    /* Check the unsatisfiability of  $\Psi \wedge \neg \varphi$  */
38:     $(res, trace) := \text{VERIFY}(\Psi, \varphi)$ 
39:  end while
40:  /* Program is still not side-channel free */
41:  /* Refine abstraction to repeat verification loop */
42:  if  $(res = false)$  then
43:     $\text{ABSREFINE}(\Psi, Pred, Pred_{cur}, trace, \Gamma)$ 
44:     $\text{MONITORING}(\Psi, O, \varphi, Pred, Pred_{cur}, \Gamma)$ 
45:  end if
46: end procedure
47: procedure ABSREFINE( $\Psi, Pred, Pred_{cur}, trace, \Gamma$ )
48:   /* Extract unsatisfiable core */
49:    $\mathcal{U} := \text{UNSATCORE}(trace, \Gamma)$ 
50:   /* Refine abstractions (see Section 4) */
51:    $Pred_{cur} := \text{REFINE}(Pred_{cur}, \mathcal{U}, Pred)$ 
52:   /* Rewrite  $\Psi$  with the refined abstraction */
53:    $\text{REWRITE}(\Psi, Pred_{cur})$ 
54: end procedure
```

---

- $Pred$  and  $Pred_{cur}$ : Cache semantics related predicates ( $Pred$ ) and the current level of abstraction ( $Pred_{cur}$ ), and
- $\Gamma$ : Symbolic conditions to determine the cache behaviour.

## Additional Experimental Results

**Sensitivity w.r.t. cache.** Figure 4 outlines the evaluation for routines that violate side-channel freedom and for attack model  $O_{time}$ . Nevertheless, the conclusion holds for all routines and attack models. Figure 4 captures the number of equivalence classes explored (hence, the number of patches generated cf. Algorithm 3) with respect to time. We make the following crucial observations from Figure 4. Firstly, the scalability of our checker is stable across a variety of cache configurations. This is because we encode cache semantics within a program via symbolic constraints on cache conflict. The size of these constraints depends on the number of memory-related instructions, but its size is not heavily influenced by the size of the cache. Secondly, the number of equivalence classes of observations does not vary significantly across cache configurations. Indeed, the number of equivalence classes may even increase (hence, increased channel capacity) with a bigger cache size (e.g. in DES and AES). However, for all cache configurations, CACHEFIX generated all the patches that need to be applied for making the respective programs cache side-channel free.

*The scalability of CacheFix is stable across a variety of cache configurations. Moreover, in all cache configurations, CacheFix generated all required patches to ensure the cache side-channel freedom w.r.t.  $O_{time}$ .*

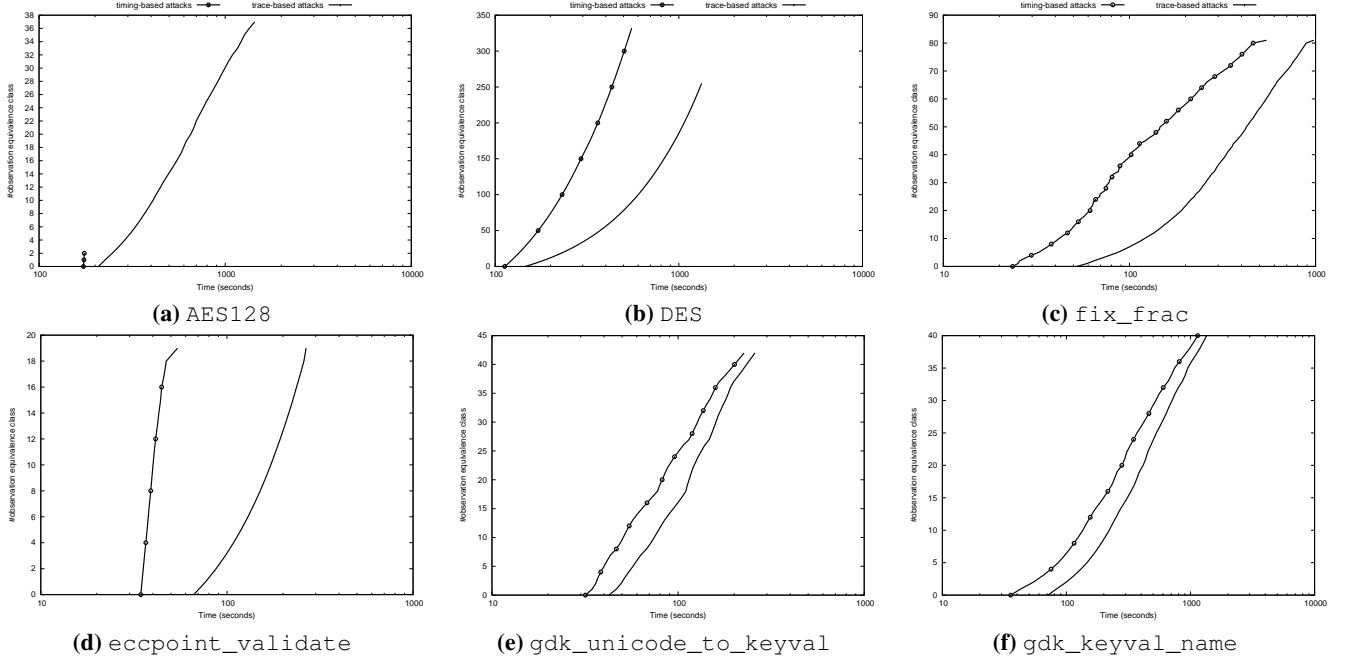

Figure 3: Overhead of counterexample exploration and patch synthesis

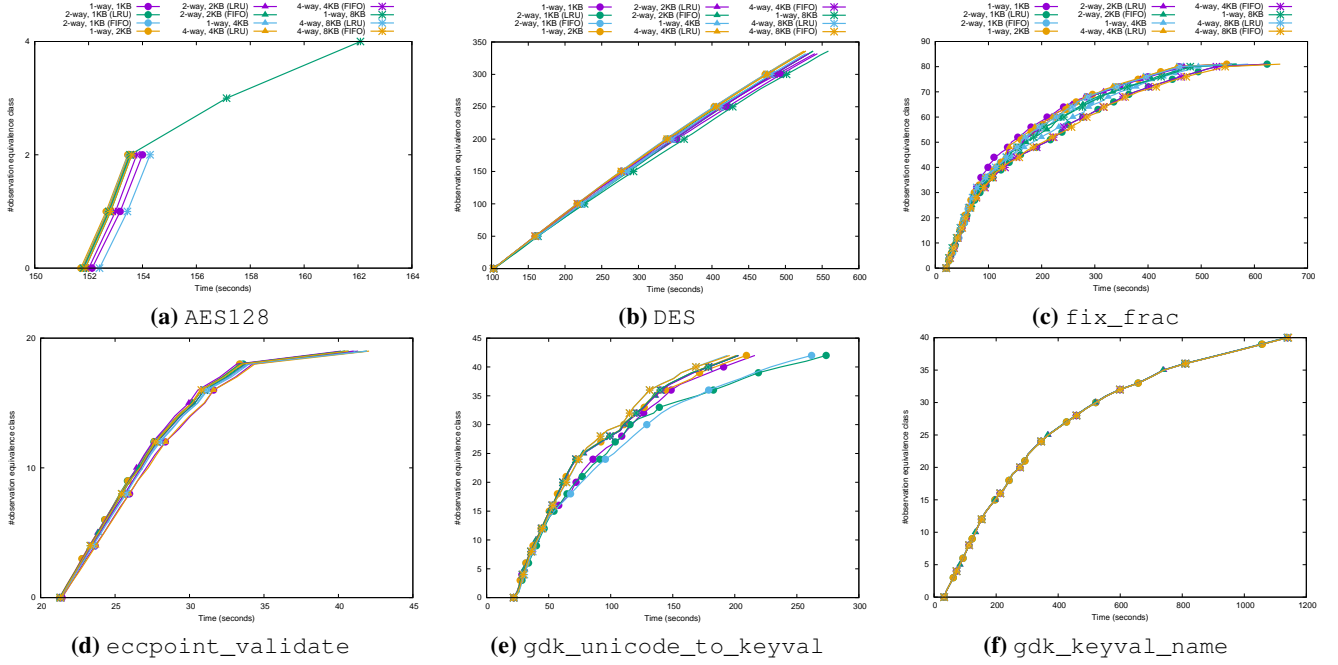

Figure 4: CACHEFIX sensitivity w.r.t. cache
